# Supplementary material for: Probabilistic Hierarchical Forecasting with Deep Poisson Mixtures
Source: arXiv:2110.13179 source file (2023-04-11)
Supplement: Supplementary file 1 [file architecture.tex]

The \MQForecaster \ architecture is based on \emph{Sequence-to-Sequence with Context} network (\SeqtoSeqC, \cite{cho2014Seq2SeqC}). The key differences are that the MQ-Forecaster uses temporal convolutions (\TemporalConv, \cite{vandenoord2016wavenet,zico2018tcnn}) to encode the available history into hidden states. And second, it uses forked decoders based on \emph{multi-layer perceptrons} (\MLP; \cite{rosenblatt1961principles}), in a direct \emph{multi-horizon forecast strategy} \citep{atiya2016multi_step_forecasting}. We describe below in further detail the components of the model.
% 1)  rather than an \LSTM, 2) , that instead of using an \LSTM \ recursive decoder.

\subsubsection{Encoder}

As explained earlier the \MQForecaster \ main encoder is a stack of  dilated temporal convolutions. Additionally we use a global dense layer to encode the static features and a local dense layer, shared across time, to encode the available future information. The encoder and its components are described in Equation~(\ref{equation:encoders}). 

\begin{equation}
\begin{aligned}
    \mathbf{h}^{(p)}_{t}  &= \mathbf{TemporalConv}(\mathbf{x}^{(p)}_{[b][:t]}) \\
    \mathbf{h}^{(f)}_{t}  &= \mathbf{MLP}_{L}(\mathbf{x}^{(f)}_{[b][t:t+h]}) \quad \qquad \qquad
    \mathbf{h}^{(s)}      = \mathbf{MLP}(\mathbf{x}^{(s)}_{[b]}) \\
    \mathbf{h}_{t}        &\equiv  \mathbf{Encoder}(\mathbf{x}^{(h)}_{[b][:t]},\;\mathbf{x}^{(f)}_{[b][t:t+h]},\;\mathbf{x}^{(s)}_{[b]})
    = [ \mathbf{h}^{(h)}_{t} |\; \mathbf{h}^{(f)}_{t} |\; \mathbf{h}^{(s)} ] \\
    \label{equation:encoders}
\end{aligned}
\end{equation}

The output of the encoder block $\mathbf{h}_{t}$, is created by concatenating the encoded past data $\mathbf{h}^{(p)}_{t}$, the encoded future information $\mathbf{h}^{(f)}_{t}$ and the encoded static features $\mathbf{h}^{(s)}$.

\subsubsection{Forked Decoders}

The \MQForecaster \ uses a two-branch \MLP \ decoder. The first (global) branch, summarizes the encoder output and future available information into two contexts. The horizon-agnostic context $\mathbf{c}_{a}$ captures common data across the forecast horizon. The horizon-specific context $\mathbf{c}_{[t:t+h]}$ provides structural awareness of the distance between the forecast creation date and the specific horizon and plays a crucial role in expressing seasonalities. It is described in Equation~(\ref{equation:forked_decoders1}).

\begin{equation}
\begin{aligned}
    \mathbf{c}_{a} &= \mathbf{MLP}(h_{t}) \qquad \qquad \qquad \qquad \qquad \mathbf{c}_{[t:t+h]} = \mathbf{MLP}_{L}(h_{t}) \\
    \label{equation:forked_decoders1}
\end{aligned}
\end{equation}    

The second (local) branch, described in Equation~(\ref{equation:forked_decoders2}), combines the horizon-agnostic and horizon-specific contexts and inputs of the original corresponding future information. Its role is to refine the resolution and
map the seasonalities into the predictions.

\begin{equation}
\begin{aligned}
    \mathbf{w}_{[k]} &= \mathrm{SoftMax}(\mathbf{MLP}(\mathbf{c}_{a})) \qquad \qquad \blambda_{[b][k][t:t+h]} = \mathbf{MLP}_{L}(\mathbf{c}_{a},\, \mathbf{c}_{[t:t+h]},\, \mathbf{x}^{(f)}_{[t:t+h]}) \\
    \label{equation:forked_decoders2}
\end{aligned}
\end{equation}

Finally, the \emph{forking sequences} technique operates a series of decoders with shared parameters at each time point $t$ of the encoded temporal data. In practice, it implements highly efficient rolling-window predictions.
