# Supplementary material for: Probabilistic Hierarchical Forecasting with Deep Poisson Mixtures
Source: arXiv:2110.13179 source file (2023-04-11)
Supplement: Supplementary file 2 [file pmm_properties.tex]

%===============================================================
\subsection{Poisson Mixture Mesh Properties}
\label{section:pmm_properties}
%===============================================================

To describe the joint distribution across all levels of the hierarchical time series structure we assume that for a given time series $\mathbf{y}_{b,[t]}$, its non overlapping observations are distributed Poisson mixture, denoted $y_{b,\,t} \sim \mathrm{PM}(\mathbf{w}_{[k]}, \blambda_{b,[k],t})$, the observations are conditionally independent given the Poisson rates, the mixing weights $\mathbf{w}_{[k]}$ are shared between the observations, and their respective Poisson components do not mix\footnote{The un-mixing property of the Poisson components refers to the assumption that the count populations of a given Poisson component are deterministic.}, under these assumptions we show in \ref{unmixing_property}, \ref{joint_distribution} and \ref{agg_rules} the properties are summarized in Table \ref{table:pmm_properties}:
\vspace{2mm}

%\newpage
\subsubsection{Unmixing Property}
\label{unmixing_property}

To describe the joint distribution across all levels of the time series structure we assume that for a given time series $\mathbf{y}_{b,[t]}$ with non overlapping observations $y_{b,\,t} \sim \mathrm{PM}(\mathbf{w}_{[k]}, \blambda_{b,[k],t})$, the observations are conditionally independent once the Poisson rates are known, the mixing weights $\mathbf{w}_{[k]}$ are shared between the observations, and their respective Poisson components do not mix. We prove the properties from Table \ref{table:pmm_properties}.

\begin{figure}[!htp]
\centering
\includegraphics[width=75mm]{images/model_graphical_b&w.pdf}
\caption{Representation of the un-mixing property of the Poisson components of the PMM.}
\end{figure}

\subsubsection{Joint Distribution}
\label{joint_distribution}

Let two bottom random variables have a PM distribution with mixing weights  $\mathbf{w}_{[k]}$ and rates $\blambda_{b,[k],t}, \blambda_{b,[k],t'}$, that is $y_{b,t} \sim \mathrm{PM}(\mathbf{w}_{[k]}, \blambda_{b,[k],t})$ and $y_{b,t'} \sim \mathrm{PM}(\mathbf{w}_{[k]}, \blambda_{b,[k],t'})$, then under the conditional independence assumption, the independence between the weights and the bottom series and the deterministic evolution property the joint distribution of the variables is:
\begin{equation*}
\begin{split}
    \mathrm{P}(y_{b,t}, y_{b,t'}) = \sum_{k} w_{k} \text{Poisson}(y_{b,t}|\;\lambda_{b,k,t}) \text{Poisson}(y_{b,t'}|\;\lambda_{b,k,t'})
\end{split}
\end{equation*}

\textit{Proof}
\begin{equation*}
\begin{split}
   \mathrm{P}(y_{b,t}, y_{b,t'}) &= \sum_{k}\sum_{l} \mathrm{P}(y_{b,t},\,y_{b,t'}|\;\lambda_{b,k,t},\lambda_{b,l,t'})\mathrm{P}(\lambda_{b,k,t}|\lambda_{b,l,t'})\mathrm{P}(\lambda_{b,l, t'}) \\
    &= \sum_{k} \mathrm{P}(y_{b,t}|\;\lambda_{b,k,t}) \mathrm{P}(y_{b,t'}|\;\lambda_{b,k,t'}) \mathrm{P}(\lambda_{b,k,t'}) \\
    &= \sum_{k} w_{k} \text{Poisson}(y_{b,t}|\;\lambda_{b,k,t}) \text{Poisson}(y_{b,t'}|\; \lambda_{b,k,t'})
\end{split}
\end{equation*}

The first equality is the chain rule of probability, the second equality comes from the deterministic evolution property, the final part comes from the conditional independence property. By induction,
$$\mathrm{P}(\mathbf{y}_{b,[t]}) = 
\sum^{N_{\lambda}}_{k=1} w_{k} \prod^{N_{T}}_{t=1} \text{Poisson}(y_{b,\,t}|\;\lambda_{b,k,t})$$

\subsubsection{Covariance Structure}
\label{section:covariance_proof}
From the joint distribution for $y_{b,t},\, y_{b,t'}$ it can be shown using linearity of expectation and the Poisson distribution properties that the covariance structure of the bottom series can be described by the covariance structure of the Poisson rates:
$$\mathrm{Cov}(y_{b,t} ,\, y_{b,t'}) = 
\sum^{N_{\lambda}}_{k=1} w_{k} (\lambda_{b,k,t}-\bar{\blambda}_{b,[k],t})(\lambda_{b,k,t'}-\bar{\blambda}_{b,[k],t'})$$
where $\bar{\blambda}_{b,[k],t}=\sum_{k}w_{k}\lambda_{b,k,t}$ and $\bar{\blambda}_{b,[k],t'}=\sum_{k}w_{k}\lambda_{b,k,t'}$. This shows that in spite of the strong assumptions made for the PMM the model is capable of describing a rich correlation structure from the dispersion inherited of the mixture.

\subsubsection{Aggregation Rule}
\label{agg_rules}

Let two bottom level random variables have a PM distribution with mixing weights $\mathbf{w}_{[k]}$ and rates $\blambda_{b,[k],t},\, \blambda_{b',[k],t}$, that is $y_{b,t} \sim \mathrm{PM}(\mathbf{w}_{[k]}, \blambda_{b,[k],t})$ and $y_{b',t} \sim \mathrm{PM}(\mathbf{w}_{[k]}, \blambda_{b',[k],t})$, then under the conditional independence assumption, the independence between the weights and the bottom series and the deterministic evolution property we have the following aggregation rule:
\[\mathbf{y}_{b,t}+\mathbf{y}_{b',t} \sim \mathrm{PM}(\mathbf{w}_{[k]}, \blambda_{b,[k],t} + \blambda_{b',[k],t})\]
\textit{Proof}
\begin{equation*}
\begin{split}
    \mathrm{P}(y_{b,t}+y_{b',t}) &=
    \sum_{k}\sum_{l} \mathrm{P}(y_{b,t}+y_{b',t}|\;\lambda_{b,k,t},\lambda_{b',l,t})\mathrm{P}(\lambda_{b,k,t}|\lambda_{b',l,t})P(\lambda_{b',l,t}) \\
    &= \sum_{k} \mathrm{P}(y_{b,t}+y_{b',t}|\;\lambda_{b,k,t},\,\lambda_{b',k,t})P(\lambda_{b',k,t}) \\
    &= \sum_{k} w_{k}\text{Poisson}(y_{b,t}+y_{b',t}|\;\lambda_{b,k,t}+\lambda_{b',k,t})
\end{split}
\end{equation*}

The first equality is the chain rule of probability, the second equality comes from the deterministic evolution property of the Poisson mixture, along with the independence of the weights from the Poisson sub population the last equality comes from the conditional independence property and the fact that the sum of independent Poisson variables is Poisson with the sum of the rates. By induction this property can be extended to its matrix with the hierarchical summation matrix $\mathbf{S}_{\mathrm{[a][b]}} \in \mathbb{R}^{N_{a} \times N_{b}}$.
$$\mathbf{y}_{[a],\,t} = 
\mathbf{S}_{\mathrm{[a][b]}}\mathbf{y}_{[b],t} \sim \mathrm{PM}(\mathbf{w}_{[k]}, \mathbf{S}_{\mathrm{[a][b]}}\blambda_{[b][k],t})$$

\begin{table*}[ht]
	\centering
	\caption{Summary properties of the Poisson Mixture Mesh distribution}
	\label{table:pmm_properties}	
	\begin{tabular}{|ll|}
		\hline
		&           \\
		1. Marginal distribution                & $y_{b,t} \sim \mathrm{PM}(\mathbf{w}_{[k]}, \blambda_{b,[k],t})$ \\
		&           \\
		2. Assumptions                          &            \\
		&           \\
		$\;$ 2.1 Conditional Independence    & $y_{b_1,t} | \lambda_{b_1,k,t} $
		$\quad
		\perp\!\!\!\perp \quad y_{b_2,t} | \lambda_{b_2,h,t}\quad$ if $b_{1},b_{2}$ do not overlap \\
		&           \\
		$\;$ 2.2 Unmixing property           & $\mathrm{P}(\lambda_{b,k,t} | 
		\lambda_{b,h,t}) = \delta_{k,h}\quad$ Poisson components do not mix \\
		&
		where $\delta_{k,h}$ representing the Kronecker delta \\
		&           \\
		3. Joint Distribution                   &
		$\mathrm{P}(\mathbf{y}_{b,[t]}) = 
		\sum^{N_{\lambda}}_{k=1} w_{k} \prod^{N_{T}}_{t=1} \text{Poisson}(y_{b,\,t}|\;\lambda_{b,k,t})$ \\
		&           \\ 
		4. Hierarchical Coherence &            \\
		&           \\
		$\;$ 4.1 Aggregation Rule            & $\mathbf{y}_{[a],\,t} = 
		\mathbf{S}_{\mathrm{[a][b]}}\mathbf{y}_{[b],t} \sim PM(\mathbf{w}_{[k]}, \mathbf{S}_{\mathrm{[a][b]}}\blambda_{[b][k],t})$ \\
		&           \\
		$\;$ 4.2 Disaggregation Rule           &
		$\mathbf{y}_{[b],\,t} = \mathbf{p}_{[b], t} \odot y_{\mathrm{Total},t} \sim \mathrm{PM}( \mathbf{w}_{[k]}, \mathbf{p}_{[b],t} \odot \blambda_{\mathrm{Total},[k],t}) \; )$ \\
		&
		with shares $0 \leq p_{b_{i}}$, $\sum_{b_{i}} p_{b_{i},t} = \mathbbm{1}$ and $\odot$  \\
		& multiplication in the b-th dimension \\
		&           \\
		5. Covariance Structure                 &
		$\mathrm{Cov}(y_{b,t} ,\, y_{b,t'}) = 
		\sum^{N_{\lambda}}_{k=1} w_{k} (\lambda_{b,k,t}-\bar{\blambda}_{b,[k],t})(\lambda_{b,k,t'}-\bar{\blambda}_{b,[k],t'})$ \\  
		&    \\ \hline  
	\end{tabular}
\end{table*}
