# Supplementary material for: Probabilistic Hierarchical Forecasting with Deep Poisson Mixtures
Source: arXiv:2110.13179 source file (2023-04-11)
Supplement: Supplementary file 3 [file qualitative_predictions.tex]

%========================================================================
\onecolumn
\section{Deep Poisson Mixture Network Forecasts comparison}
\label{section:forecasts_comparison}
%=======================================================================

\vspace{5mm}
\subsection{DPMN Naive Bottom Up Forecasts}

As mentioned in Section~\ref{section:estimation_inference}, composite likelihood may suffer from model misspecification. The \ours-\NaiveBU \ does not learn the dependencies or correlations between time-series in the hierarchy. As shown in Figure~\ref{fig:pmmcnn_naivebu_hierarchical_predictions} the \ours-\NaiveBU \ produces \EDITtwo{forecast} distributions for the aggregate levels unnecessarily wide, as it pushes the limits of the aggregation rule.

Still, the \ours-\NaiveBU \ performs well in disaggregated series and means as we show in the empirical evaluation of Section~\ref{section:experiments}. The \ours-\NaiveBU \ produces \EDITtwo{forecasts} comparable to those of statistical alternatives on the \TourismL \ and \Favorita \ datasets and outperforms all the other algorithms in the \Traffic \ dataset where the hierarchical structure is noisy or not as informative.

\begin{figure*}[ht]
\centering
\includegraphics[width=0.95\linewidth]{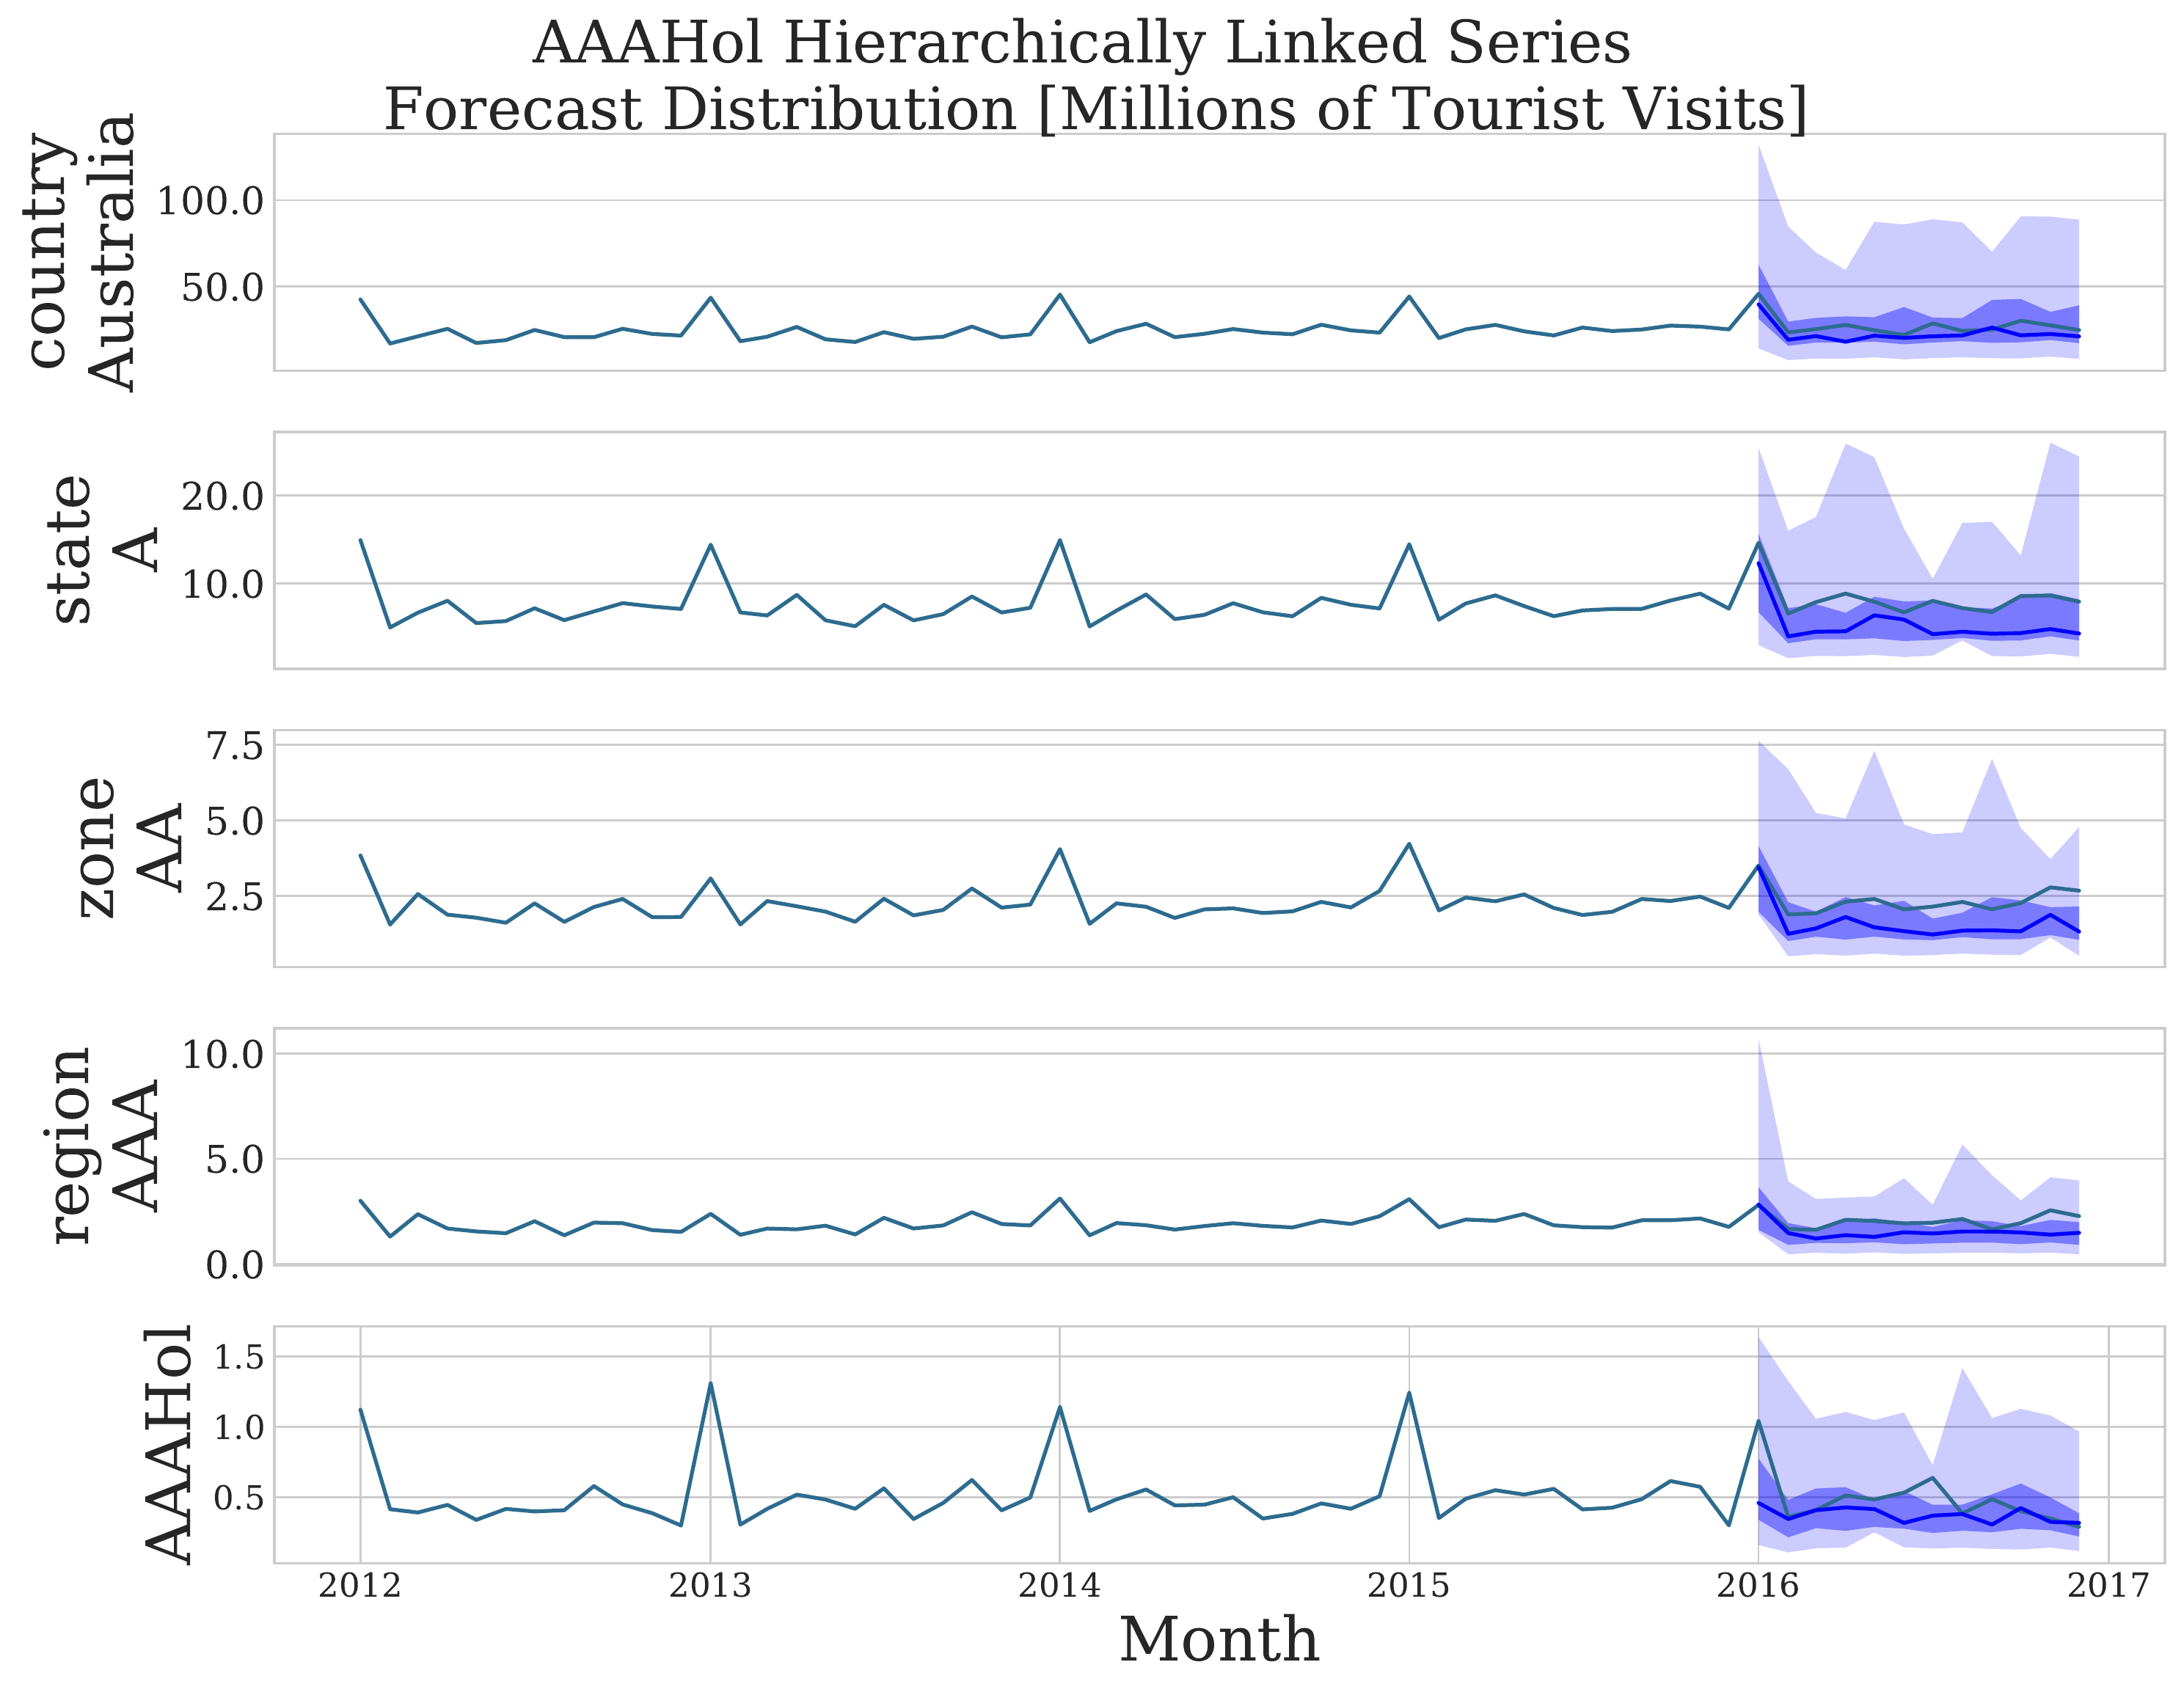}
\caption{\ours-\NaiveBU \ predictive distributions on a hierarchically linked time series from the \TourismL \ dataset. The top row shows the total number of tourist visits in Australia (TotalAll), the second row shows the visits to Australia for the North South Wales state (AAll), the third row shows the holiday visits in the metropolitan Area of New South Wales (AAAll), the fourth row shows the holiday visits in Sidney (AAAAll), the final row shows the holiday visits to Sidney. Quantile \EDITtwo{forecasts} are shown in colored lines.} \label{fig:pmmcnn_naivebu_hierarchical_predictions}
\end{figure*}

\clearpage
\vspace{10mm}
\subsection{DPMN Group Bottom Up Forecasts}

The \GroupBU \ composite likelihood estimation method considers dependencies and correlations between time series.  When in the presence of informative time-series group structures, the \ours-\GroupBU \ uses the expressiveness of the multivariate Poisson joint distribution to its advantage. It better models the dependencies within the time-series groups it considers during its estimation while remaining computationally tractable.

As we show in Section~\ref{section:experiments} and Figure~\ref{fig:pmmcnn_groupbu_hierarchical_predictions} when in the presence of strong correlation structures between the time series, like the ones in the \TourismL \ and \Favorita \ datasets, the \ours-\GroupBU \ outperforms all the hierarchical forecasting alternatives that we considered in our experiments. However, we showcase the limits of the method when the groups of series considered by the model are noisy or as informative as the case of the \Traffic \ dataset where the group structure was randomly assigned.

\begin{figure*}[ht]
\centering
\includegraphics[width=0.95\linewidth]{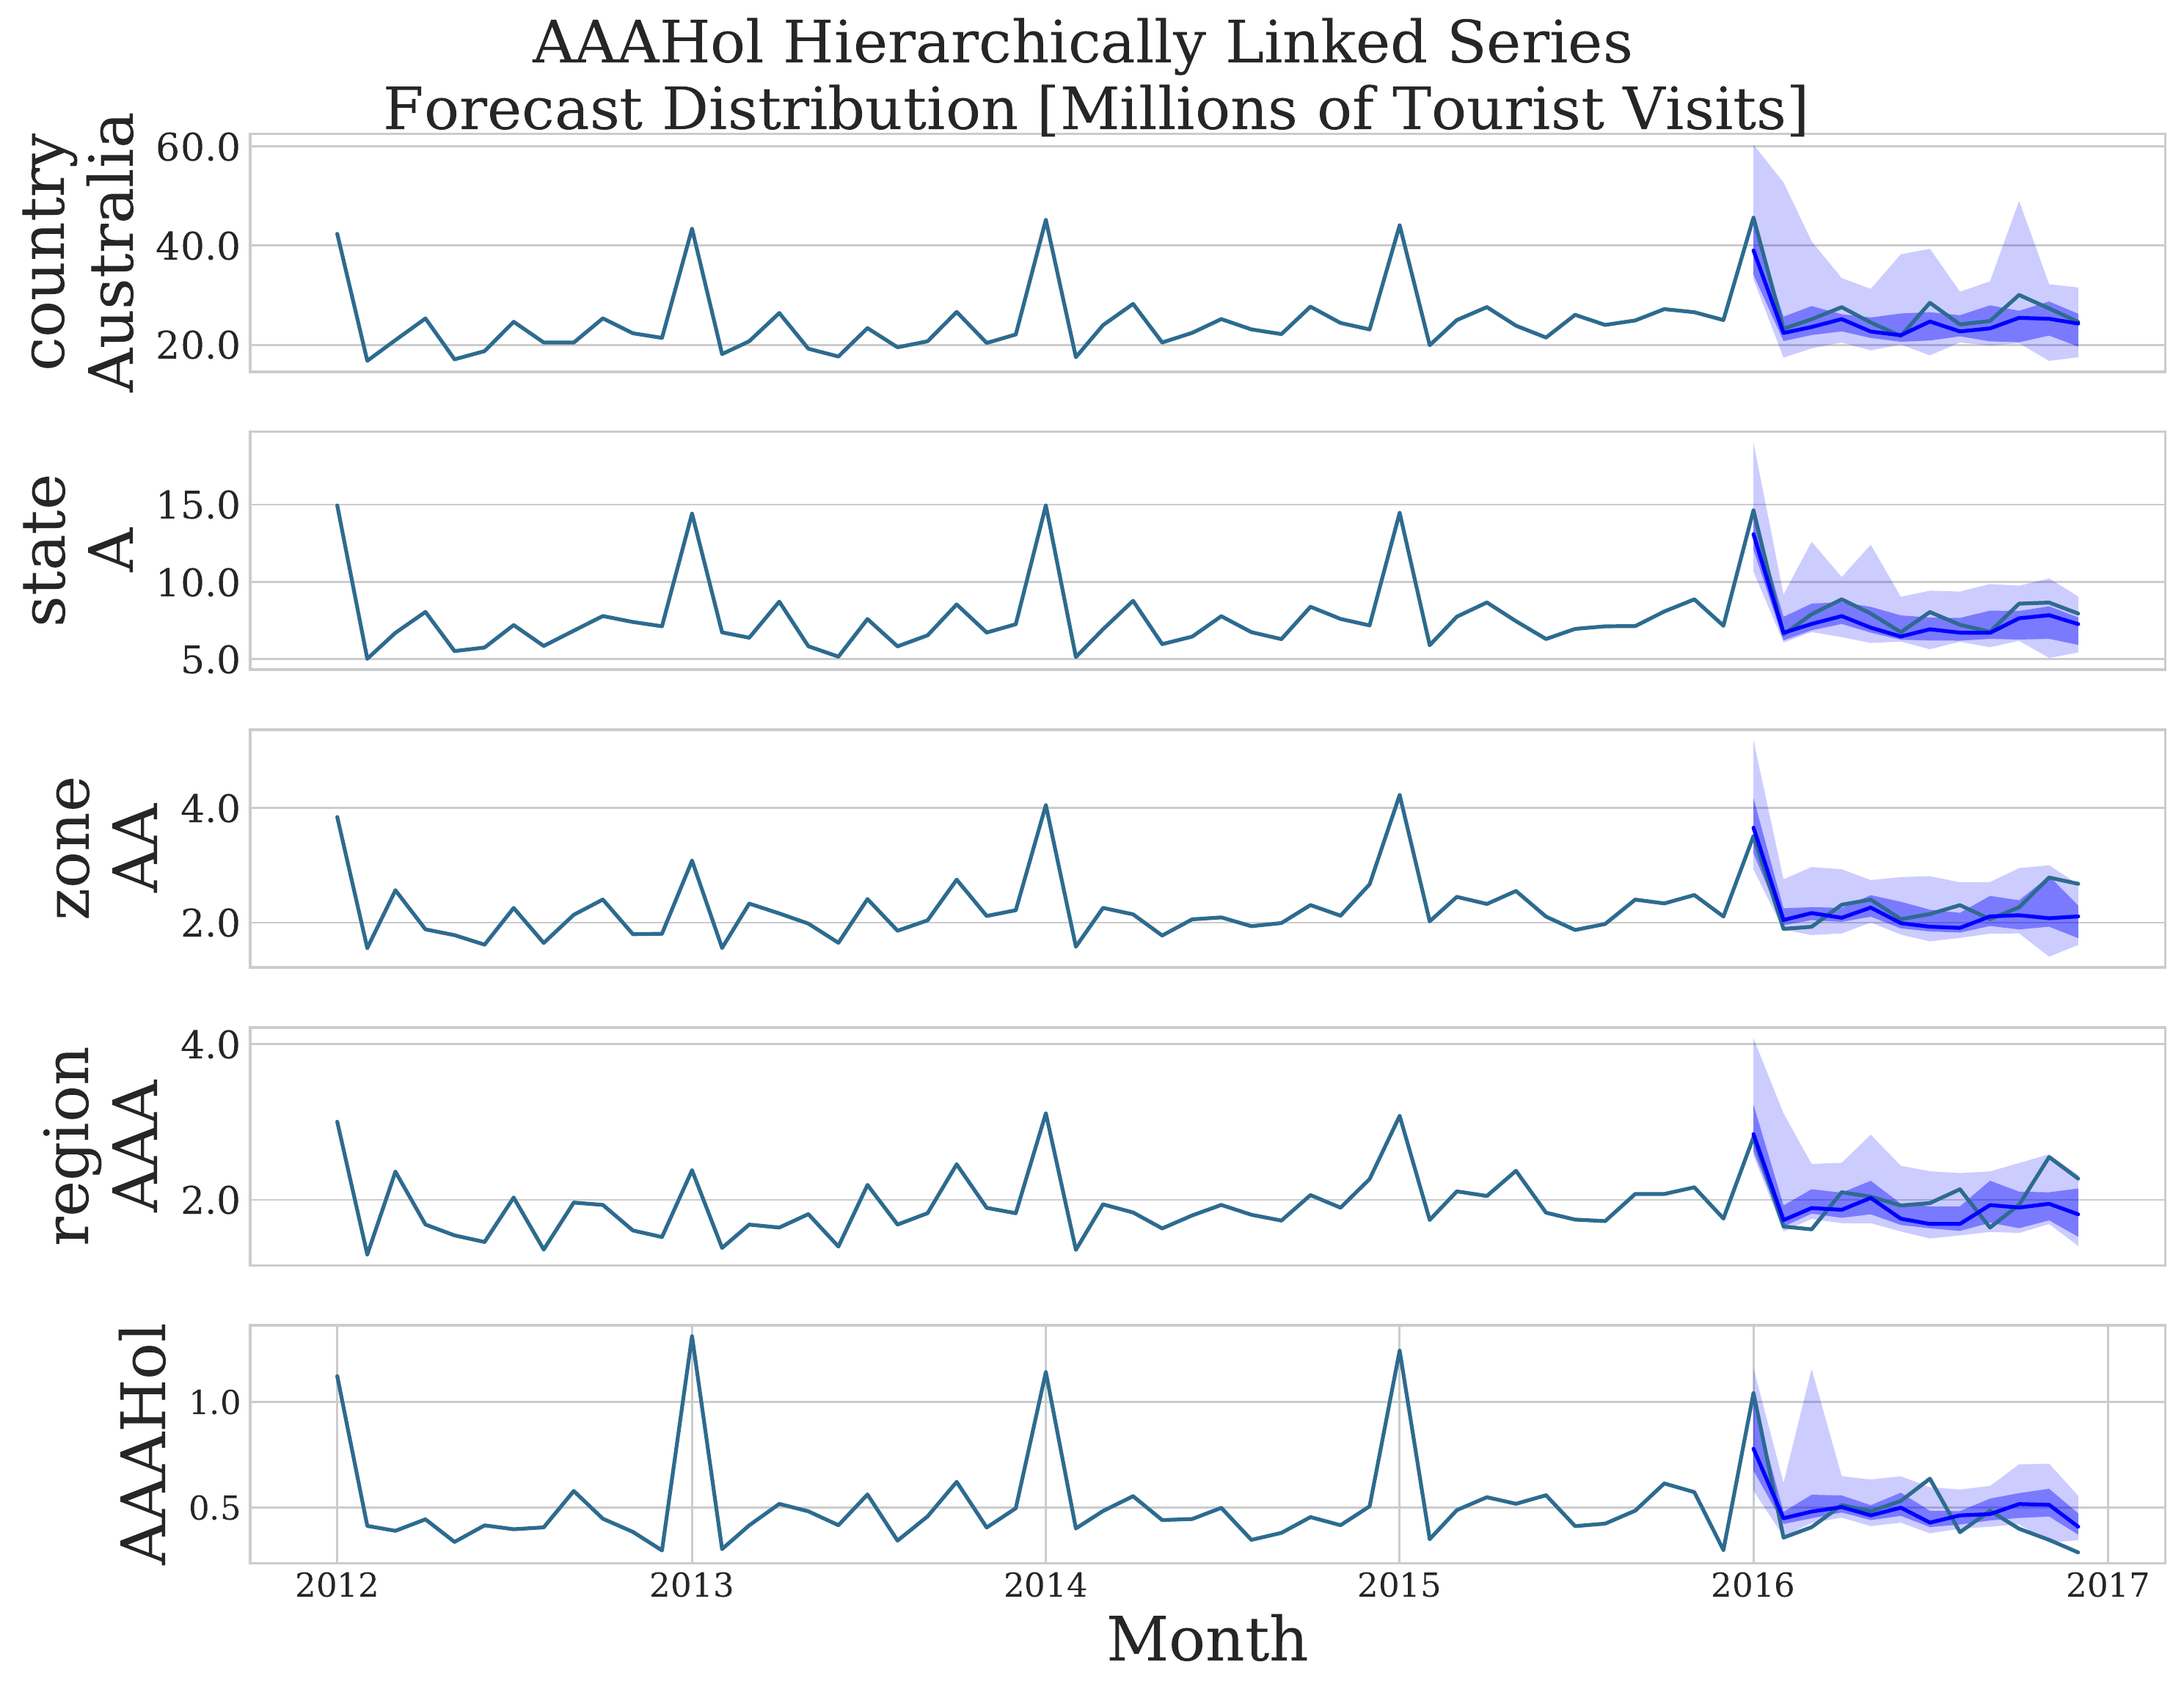}
\caption{\ours-\GroupBU \ predictive distributions on a hierarchically linked time series from the \TourismL \ dataset. The top row shows the total number of tourist visits in Australia (TotalAll), the second row shows the visits to Australia for the North South Wales state (AAll), the third row shows the holiday visits in the metropolitan Area of New South Wales (AAAll), the fourth row shows the holiday visits in Sidney (AAAAll), the final row shows the holiday visits to Sidney. Quantile \EDITtwo{forecasts} are shown in colored lines.} \label{fig:pmmcnn_groupbu_hierarchical_predictions}
\end{figure*}
